# Supplementary material for: CacheGen: KV Cache Compression and Streaming for Fast Large Language Model Serving
Source: arXiv:2310.07240 source file (2024-07-19)
Supplement: Supplementary file 2 [file revision-appendix.tex]

\onecolumn % to fit tabularx 

\section*{Appendix. }
\label{sec:revision}

\section*{Labels included in each subcategory} 

\subsection{}
